# Supplementary material for: Quantum Information Fusion and Correction under the Transferable Belief Model
Source: arXiv:2410.08949 source file (2026-08-22)
Supplement: Supplementary file 1 [file supplementary.pdf]

# Supplementary Material for Transferable Belief Model on Quantum Circuits

October 17, 2024

**Theorem 1.** *To implement the poss-transferable mass function within an  $n$ -element FoD, only  $n$  RY gates are required to implement its quantum state, with the parameter  $\theta$  determined by its contour function.*

*Proof.* Consider a poss-transferable mass function  $m_{Poss}$  under an  $n$ -element FoD, its contour function is denoted as  $pl_{Poss}$ . For an  $n$ -qubit systems with initial state  $|0\rangle^n$ , its qubits are denoted as  $q_0, \dots, q_{n-1}$ . For the  $k$  from 0 to  $n-1$ , apply the  $R_Y(\theta_{k+1})$  gate on  $q_k$ , where  $\theta_{k+1} = \arctan \sqrt{\frac{pl_{Poss}(\omega_{k+1})}{1-pl_{Poss}(\omega_{k+1})}}$ , the state's evolution is

$$|0\rangle^n \rightarrow \sum_{i=0:2^n-1} \sqrt{\prod_{\omega \in F_i} pl_{Poss}(\omega) \prod_{\omega \notin F_i} (1-pl_{Poss}(\omega))} |\text{bin}(i)\rangle \rightarrow \sum_{F_i \subseteq \Omega} \sqrt{m_{Poss}(F_i)} |\text{bin}(i)\rangle = |m_{Poss}\rangle.$$

Hence,  $n$  RY gates can implement the poss-transferable mass function on quantum circuits, and the parameters are related to its contour function.  $\square$

**Theorem 2.** *For the same Boolean algebra operation  $\mathfrak{B}$ , the square of amplitude of  $|m_{k+1}\rangle$  in Definition 6 equals the outcome  $m_{k+1}$  in Definition 5.*

*Proof.* The BACR can be divided into multiple sub-processes based on layers and operation components, and the combination of these sub-processes can also be considered a BACR. Hence, if this theorem is proven for a BACR with only one operation, i.e., no ancilla qubits are required, it can be generalized to the general BACR. Suppose the Boolean algebra operation satisfies  $\mathfrak{B}(F_{i_1}, \dots, F_{i_k}) = F_{i_{k+1}}$ , the specific evolutionary process on quantum circuit is:

- Prepare the initial state:

$$|m_1\rangle \cdots |m_k\rangle |0\rangle^n = \sum_{F_{i_1} \subseteq \Omega} \cdots \sum_{F_{i_k} \subseteq \Omega} \prod_{j=1}^k \sqrt{m_j(F_{i_j})} |\text{bin}(i_1)\rangle \cdots |\text{bin}(i_k)\rangle |0\rangle^n.$$

- Apply the corresponding gates to implement the  $\mathfrak{B}$  on the element  $\omega_n$ , which correspond to qubits  $q_{n-1}$ s, where control bits are  $q_{n-1_1} \cdots q_{n-1_k}$  and target bit is  $q_{n-1_{k+1}}$ , and the above state evolves as:

$$\begin{aligned} & \sum_{\mathfrak{B}(q_{n-1_1}, \dots, q_{n-1_k}) = q_{n-1_{k+1}} = 0} \sum_{F_{i_1} \subseteq \Omega} \cdots \sum_{F_{i_k} \subseteq \Omega} \prod_{j=1}^k \sqrt{m_j(F_{i_j})} |\text{bin}(i_1)\rangle \cdots |\text{bin}(i_k)\rangle |0\rangle^n + \\ & \sum_{\mathfrak{B}(q_{n-1_1}, \dots, q_{n-1_k}) = q_{n-1_{k+1}} = 1} \sum_{F_{i_1} \subseteq \Omega} \cdots \sum_{F_{i_k} \subseteq \Omega} \prod_{j=1}^k \sqrt{m_j(F_{i_j})} |\text{bin}(i_1)\rangle \cdots |\text{bin}(i_k)\rangle |1\rangle |0\rangle^{n-1}. \end{aligned}$$

- Continue to implement the  $\mathfrak{B}$  on the elements  $\omega_0 \cdots \omega_{n-1}$ , the evolved state is:

$$\begin{aligned} & \sum_{\mathfrak{B}(q_{n-1_1}, \dots, q_{n-1_k}) = 0} \cdots \sum_{\mathfrak{B}(q_{0_1}, \dots, q_{0_k}) = 0} \sum_{F_{i_1} \subseteq \Omega} \cdots \sum_{F_{i_k} \subseteq \Omega} \prod_{j=1}^k \sqrt{m_j(F_{i_j})} |\text{bin}(i_1)\rangle \cdots |\text{bin}(i_k)\rangle |0\rangle^n + \\ & \sum_{\mathfrak{B}(q_{n-1_1}, \dots, q_{n-1_k}) = 0} \cdots \sum_{\mathfrak{B}(q_{0_1}, \dots, q_{0_k}) = 1} \sum_{F_{i_1} \subseteq \Omega} \cdots \sum_{F_{i_k} \subseteq \Omega} \prod_{j=1}^k \sqrt{m_j(F_{i_j})} |\text{bin}(i_1)\rangle \cdots |\text{bin}(i_k)\rangle |0\rangle^{n-1} |1\rangle + \\ & \cdots + \sum_{\mathfrak{B}(q_{n-1_1}, \dots, q_{n-1_k}) = 1} \cdots \sum_{\mathfrak{B}(q_{0_1}, \dots, q_{0_k}) = 1} \sum_{F_{i_1} \subseteq \Omega} \cdots \sum_{F_{i_k} \subseteq \Omega} \prod_{j=1}^k \sqrt{m_j(F_{i_j})} |\text{bin}(i_1)\rangle \cdots |\text{bin}(i_k)\rangle |1\rangle^n. \end{aligned}$$

Consider a focal set  $F_{i_{k+1}}$ , whose belief masses in Definition 5 is

$$m_{k+1}(F_{i_{k+1}}) = \sum_{\mathfrak{B}(F_{i_1}, \dots, F_{i_k}) = F_{i_{k+1}}} \prod_{j=1}^k m_j(F_{i_j}),$$

and the amplitude of  $|\text{bin}(i_{k+1})\rangle$  in the above state is

$$\sqrt{\sum_{\mathfrak{B}(F_{i_1}, \dots, F_{i_k}) = F_{i_{k+1}}} \prod_{j=1}^k m_j(F_{i_j})} |\text{bin}(i_{k+1})\rangle.$$

Hence, the proposed approach in Definition 6 can implement the BACR on quantum circuits without theoretical errors.  $\square$

**Theorem 3.** *The CECR and DECR from two sources can be implemented on quantum circuit without ancilla bits, which is more efficiently than the evolution proposed in Definition 6.*

*Proof.* Consider two mass functions  $m_1$  and  $m_2$  under an  $n$ -element FoD  $\Omega$ , whose MFQSSs, denoted as  $|m_1\rangle$  and  $|m_2\rangle$ , are implemented on qubits  $q_0, \dots, q_{n-1}$ , ( $t = \{1, 2\}$ ). When the state is performed on circuit in Figure 1,

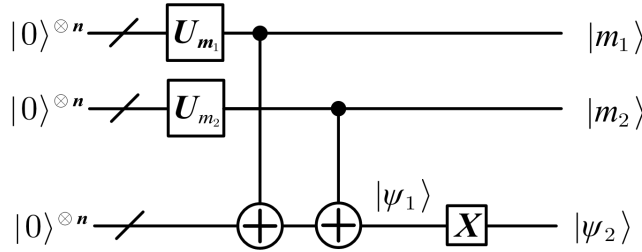

Figure 1: Implementation of DECR and CECR on quantum circuit.

the specific evolutionary process is:

- Prepare the initial state:  $\sum_{F_{i_{t1}} \subseteq \Omega} \sum_{F_{i_{t2}} \subseteq \Omega} \sqrt{m_1(F_{i_{t1}})m_2(F_{i_{t2}})} |\text{bin}(i_{t1})\rangle |\text{bin}(i_{t2})\rangle |0\rangle_{q_0, \dots, q_{n-1}}$ .
- Perform  $n$  C-NOT gates, where the control bit is  $q_{j_1}$  and the target bit is  $q_{j_3}$ , where  $j = \{0, \dots, n-1\}$ :  $\sum_{F_{i_{t1}} \subseteq \Omega} \sum_{F_{i_{t2}} \subseteq \Omega} \sqrt{m_1(F_{i_{t1}})m_2(F_{i_{t2}})} |\text{bin}(i_{t1})\rangle |\text{bin}(i_{t2})\rangle |\text{bin}(i_{t1})\rangle$ .
- Perform  $n$  C-NOT gates, where the control bit is  $q_{j_2}$  and the target bit is  $q_{j_3}$ , where  $j = \{0, \dots, n-1\}$ :

$$\begin{aligned} |\psi_1\rangle &= \sum_{F_{i_{t1}} \subseteq \Omega} \sum_{F_{i_{t2}} \subseteq \Omega} \sqrt{m_1(F_{i_{t1}})m_2(F_{i_{t2}})} |\text{bin}(i_{t1})\rangle |i_{t2}^n, \dots, i_{t2}^0\rangle \bigotimes_{p=n \rightarrow 1} \begin{cases} i_{t1}^p & i_{t2}^p = 0, \\ \neg i_{t1}^p & i_{t2}^p = 1. \end{cases} \\ &= \sum_{F_{i_{t1}} \subseteq \Omega} \sum_{F_{i_{t2}} \subseteq \Omega} \sqrt{m_1(F_{i_{t1}})m_2(F_{i_{t2}})} |\text{bin}(i_{t1})\rangle |i_{t2}^n, \dots, i_{t2}^0\rangle \bigotimes_{p=n \rightarrow 1} |(i_{t1} \wedge i_{t2}) \vee (\neg i_{t1} \wedge i_{t2})\rangle. \end{aligned}$$

- Perform  $n$  X gates on  $q_{j_3}$ , where  $j = \{0, \dots, n-1\}$ :

$$|\psi_2\rangle = \sum_{F_{i_{t1}} \subseteq \Omega} \sum_{F_{i_{t2}} \subseteq \Omega} \sqrt{m_1(F_{i_{t1}})m_2(F_{i_{t2}})} |\text{bin}(i_{t1})\rangle |i_{t2}^n, \dots, i_{t2}^0\rangle \bigotimes_{p=n \rightarrow 1} |(i_{t1} \wedge i_{t2}) \vee (\neg i_{t1} \wedge \neg i_{t2})\rangle.$$

The states of  $q_{j_3}$ , ( $j = \{0, \dots, n-1\}$ ) in  $|\psi_1\rangle$  and  $|\psi_2\rangle$  are

$$\begin{aligned} |\psi_1\rangle_{q_0, \dots, q_{n-1}} &= \sqrt{\sum_{F_{i_{t3}} = (F_{i_{t1}} \cap \overline{F_{i_{t2}}}) \cup (F_{i_{t2}} \cap \overline{F_{i_{t1}}})} m_1(F_{i_{t1}})m_2(F_{i_{t2}})} |\text{bin}(i_{t3})\rangle, \\ |\psi_2\rangle_{q_0, \dots, q_{n-1}} &= \sqrt{\sum_{F_{i_{t3}} = (F_{i_{t1}} \cap F_{i_{t2}}) \cup (\overline{F_{i_{t1}}} \cap \overline{F_{i_{t2}}})} m_1(F_{i_{t1}})m_2(F_{i_{t2}})} |\text{bin}(i_{t3})\rangle. \end{aligned}$$

It is evident that their square of amplitudes equals the outcomes of DECR and CECR, respectively, hence, the Theorem 3 is proven.  $\square$

**Theorem 4.** The  $\mathbf{K}_{F_i}^{\cup, \alpha}$  can be implemented through the Kronecker multiplication of 2-dimensional matrices. In the realm of the conjunctive case, the characteristic matrix is  $\mathbf{C}^{\cap, \alpha} = \begin{bmatrix} \alpha & 1 \\ 1 - \alpha & 0 \end{bmatrix}$ , and for the focal set  $F_i$ , the corre-

sponding matrix  $\mathbf{K}_{F_i}^{\cap, \alpha} = \bigotimes_{j=1:|\Omega|} \begin{cases} \mathbf{C}^{\cap, \alpha} & \omega_{|\Omega|-j+1} \notin F_i, \\ \mathbf{I}_2 & \omega_{|\Omega|-j+1} \in F_i. \end{cases}$  In the realm of the disjunctive case, the characteristic

matrix is  $\mathbf{C}^{\cup, \alpha} = \begin{bmatrix} 0 & 1 - \alpha \\ 1 & \alpha \end{bmatrix}$ , and for the focal set  $F_i$ , the corresponding matrix  $\mathbf{K}_{F_i}^{\cup, \alpha} = \bigotimes_{j=1:|\Omega|} \begin{cases} \mathbf{C}^{\cup, \alpha} & \omega_{|\Omega|-j+1} \in F_i, \\ \mathbf{I}_2 & \omega_{|\Omega|-j+1} \notin F_i. \end{cases}$

*Proof.* For the disjunctive case, the matrix  $\mathbf{K}_{\{\omega\}}^{\cup, \alpha} = \bigotimes_{j=1:|\Omega|} \mathbf{M}_j$ . The outcome of Kronecker multiplication is

$$K_{\{\omega\}}^{\cup, \alpha}(F_i, F_j) = \prod_{k=1:n} \begin{cases} M_k(1, 1) & \omega \notin F_i, \omega \notin F_j, \\ M_k(1, 2) & \omega \notin F_i, \omega \in F_j, \\ M_k(2, 1) & \omega \in F_i, \omega \notin F_j, \\ M_k(2, 2) & \omega \in F_i, \omega \in F_j, \end{cases} \text{ where } \mathbf{M}_k = \begin{cases} \mathbf{C}^{\cup, \alpha} & \omega = \omega_k, \\ \mathbf{I}_2 & \omega \neq \omega_k. \end{cases} \text{ Hence, the non-zero elements}$$

in  $K_{\{\omega\}}^{\cup, \alpha}(F_i, F_j)$  only appear when the elements in  $F_i$  and  $F_j$  are identical except the state of  $\omega$ , i.e.,  $F_i = F_j$ ,  $F_i = F_j \cup \{\omega\}$ ,  $F_i = F_j \setminus \{\omega\}$ . The specific cases are discussed as follows:

- When  $F_i = F_j$  and  $\omega \in F_i$ ,  $K_{\{\omega\}}^{\cup, \alpha}(F_i, F_j) = \alpha$ .
- When  $F_i = F_j$  and  $\omega \notin F_i$ ,  $K_{\{\omega\}}^{\cup, \alpha}(F_i, F_j) = 0$ .
- When  $F_i = F_j \setminus \{\omega\}$ ,  $K_{\{\omega\}}^{\cup, \alpha}(F_i, F_j) = 1 - \alpha$ .
- When  $F_i = F_j \cup \{\omega\}$ ,  $K_{\{\omega\}}^{\cup, \alpha}(F_i, F_j) = 1$ .

Hence, the  $\mathbf{K}_{\{\omega\}}^{\cup, \alpha}$  can be implemented through the above equation. According to the Eq. (6),

$$\begin{aligned} \mathbf{K}_{F_i}^{\cup, \alpha} &= \prod_{\omega \in F_i} \mathbf{K}_{\omega}^{\cup, \alpha} = \prod_{\omega \in F_i} \bigotimes_{j=1:|\Omega|} \mathbf{M}_j = \prod_{\omega \in F_i} \mathbf{I}_2 \otimes \dots \otimes \mathbf{C}^{\cup, \alpha} \otimes \dots \otimes \mathbf{I}_2 \\ &= \bigotimes_{j=1:|\Omega|} \mathbf{I}_2 \times \dots \times \mathbf{C}^{\cup, \alpha} \times \dots \times \mathbf{I}_2 = \bigotimes_{j=1:|\Omega|} \begin{cases} \mathbf{C}^{\cup, \alpha} & \omega_{|\Omega|-j+1} \in F_i, \\ \mathbf{I}_2 & \omega_{|\Omega|-j+1} \notin F_i. \end{cases} \end{aligned}$$

Similarly, the conjunctive case also can be proven through the above process, and the  $\alpha$ -junction can be implemented through Kronecker multiplications of 2-dimensional matrices.  $\square$

**Theorem 5.** For the same parameter  $\alpha$ , the  $m_{2, F_i}^{\cup, \alpha}$  of  $m$  in  $\alpha$ -junction equals the square of amplitude of  $|m_{2, F_i}^{\cup, \alpha}\rangle$  in Definition 7.

*Proof.* When there is only an element in the FoD, the classical conjunctive cases are

$$\mathbf{m}_{2, \emptyset}^{\cap, \alpha} = \begin{bmatrix} \alpha & 1 \\ 1 - \alpha & 0 \end{bmatrix} \begin{bmatrix} m_2(\emptyset) \\ m_2(\{\omega\}) \end{bmatrix} = \begin{bmatrix} \alpha m_2(\emptyset) + m_2(\{\omega\}) \\ (1 - \alpha)m_2(\emptyset) \end{bmatrix}, \quad \mathbf{m}_{2, \omega}^{\cap, \alpha} = \begin{bmatrix} 1 & 0 \\ 0 & 1 \end{bmatrix} \begin{bmatrix} m_2(\emptyset) \\ m_2(\{\omega\}) \end{bmatrix} = \begin{bmatrix} m_2(\emptyset) \\ m_2(\{\omega\}) \end{bmatrix}.$$

According to the Definition 2, the evolutionary of state is

Prepare initial state:  $\sqrt{m(\emptyset)} |0\rangle |0\rangle + \sqrt{m(\{\omega\})} |1\rangle |0\rangle$ .

Perform X gate:  $\sqrt{m(\{\omega\})} |0\rangle |0\rangle + \sqrt{m(\emptyset)} |1\rangle |0\rangle$ .

Perform Control RY gate:  $\sqrt{m(\{\omega\})} |0\rangle |0\rangle + \sqrt{m(\emptyset)} \cos(\frac{\theta}{2}) |1\rangle |0\rangle + \sqrt{m(\emptyset)} \sin(\frac{\theta}{2}) |1\rangle |1\rangle$ .

Perform X gate:  $\sqrt{m(\{\omega\})} |1\rangle |0\rangle + \sqrt{m(\emptyset)} \cos(\frac{\theta}{2}) |0\rangle |0\rangle + \sqrt{m(\emptyset)} \sin(\frac{\theta}{2}) |0\rangle |1\rangle$ .

The probabilities of measuring  $q_0$  are  $Prob(|0\rangle) = m(\emptyset)$  and  $Prob(|1\rangle) = m(\{\omega\})$ , and  $q_{0_a}$  are  $Prob(|0\rangle) = m(\emptyset)\cos^2(\frac{\theta}{2}) + m(\{\omega\})$  and  $Prob(|1\rangle) = m(\emptyset)\sin^2(\frac{\theta}{2})$ . According to the Theorem 4, since the composition of quantum systems also can be written as Kronecker multiplications, the case of singleton element can be generalized to the cases with multiple elements. The disjunctive case has the similar evolutionary process, and the Theorem 5 is proven.  $\square$

**Theorem 6.** Consider  $k$  mass functions  $m_1, \dots, m_k$  under an  $n$ -element FoD, their MFQSs are denoted as  $|m_1\rangle, \dots, |m_k\rangle$ . If the BACR with Boolean operation  $\mathfrak{B} = F_{i_1} \cap \dots \cap F_{i_k}$ , i.e., multi-source CCR, is implemented on quantum circuits, it will cost  $(k-1) \times n$  Toffoli gates.

*Proof.* According to the Definition 6, combining them via CCR needs  $n$   $C^k$ -NOT gates. In order to implement it through Toffoli gates,  $(k-1) \times n$  ancilla bits should be introduced, which is used to store the intermediate states in evolutionary processes. Hence,  $(k-1) \times n$  Toffoli gates are needed to implement the CCR of  $k$  mass functions on quantum circuits.  $\square$

**Theorem 7.** In classical works, the computational complexity of combining  $k$  mass functions under an  $n$ -element FoD using CCR depends on the types of mass functions involved. For a poss-transferable mass function, the combination requires  $(k-1) \times n$  multiplications, while for a general mass function, it requires  $(k-1) \times 2^n$  multiplications.

*Proof.* Since the poss-transferable mass function satisfies combination rule consistency, i.e.,

$$m_{Poss_1} \odot \dots \odot m_{Poss_k} = m_{Poss_1 \odot \dots \odot Poss_k}.$$

The CCR of poss-transferable mass function can be implemented through the contour functions  $pl_{k+1} = pl_1 \odot \dots \odot pl_k$ , which are  $(k-1) \times n$  multiplications are required. For the general mass functions, based on the Eq. (2), the CCR can be implement through the commonality functions  $q_{k+1} = q_1 \odot \dots \odot q_k$  with  $(k-1) \times 2^n$  multiplications.  $\square$

**Theorem 8.** Consider a mass function  $m$  under an  $n$ -element FoD, with its MFQS represented as  $|m\rangle$  in an  $n$ -qubit system. Implementing  $|m^{\cdot\alpha}\rangle$  requires  $n$  Control-RY gates, while extracting  $|m_{F_0}^{\cdot\alpha}\rangle \dots |m_{F_{2^n-1}}^{\cdot\alpha}\rangle$  requires  $n \times 2^n$  C-NOT gates.

*Proof.* According to the Definition 7, it is evident that implementing  $|m^{\cdot\alpha}\rangle$  costs  $n$  Control-RY gates and extracting the information of a focal set costs  $n$  C-NOT gates. Since there is  $2^n$  subsets in the power set, extracting information of all focal sets will cost  $n \times 2^n$  C-NOT gates.  $\square$

**Theorem 9.** Consider two mass functions,  $m_1$  and  $m_2$ , under an  $n$ -element frame of discernment, with their MFQSs represented as  $|m_1\rangle$  and  $|m_2\rangle$ . Implementing the  $\alpha$ -junction rule in Definition 8 requires  $4n$  operations.

*Proof.* According to the Definition 8, implementing the CCR or DCR costs  $n$  Toffoli gates, CCCR or DECR costs  $2n$  C-NOT gates, and adjusting the degree costs  $n$  Control RY gates. Hence, it needs  $4n$  operations to implement the entire  $\alpha$ -junction on quantum circuits.  $\square$

**Theorem 10.** In classical frameworks, the computational complexity of implementing  $\mathbf{m}_{F_i}^{\cdot\alpha}$  depends on the type of mass function. For the poss-transferable mass function, the implementations of  $\mathbf{m}_{F_0}^{\cdot\alpha}, \dots, \mathbf{m}_{F_{2^n-1}}^{\cdot\alpha}$  require  $n \times 2^n$  multiplications. For the general mass functions, the implementations of above require  $2^{2^n}$  multiplications.

*Proof.* Similar to the proof of Theorem 7, when  $m$  is a poss-transferable mass function, implementing  $\mathbf{m}_{F_i}^{\cdot\alpha}$  only requires modifying the contour functions, resulting in  $n \times 2^n$  multiplications. When  $m$  is a general mass function, implementing  $\mathbf{m}_{F_i}^{\cdot\alpha}$  requires not only modifying the contour functions but also accounting for the entanglement information in subsets with multiple elements. Consequently,  $2^{2^n}$  multiplications are required.  $\square$

**Theorem 11.** The square of amplitude output state  $|m^{\Omega \times \Theta \downarrow \Omega}\rangle$  in Definition 11 equals the outcome of marginalization in Eq. (10).

*Proof.* According to the steps in Definition 11, the specific evolutionary process is

- The MFQS of  $m^{\Omega \times \Theta}$  and the ancilla qubits compose the initial state:

$$\sum_{F_i \times G_j \subseteq \Omega \times \Theta, F_i \subseteq \Omega, G_j \subseteq \Theta} \sqrt{m^{\Omega \times \Theta}(F_i \times G_j)} |q_{(0,0)}^{(i,j)} \cdots q_{(|\Omega|-1,|\Theta|-1)}^{(i,j)} \rangle |0\rangle_{q_{0_a} \cdots q_{n-1_a}},$$

$$\text{where } q_{(s,t)}^{(i,j)} = \begin{cases} 1 & \omega_{s+1} \in F_i \text{ and } \theta_{t+1} \in G_j, \\ 0 & \text{others.} \end{cases}$$

- Perform an  $C^{|\Theta|}$ -NOT gates on the state, where the negative control bits are  $q_{(0,0)}, \dots, q_{(0,|\Theta|-1)}$  and the target bit is  $q_{0_a}$ :

$$\begin{aligned} & \sum_{q_{(0,0)}^{(i,j)} \cup \dots \cup q_{(0,|\Theta|-1)}^{(i,j)} = 1} \sum_{F_i \times G_j \subseteq \Omega \times \Theta, F_i \subseteq \Omega, G_j \subseteq \Theta} \sqrt{m^{\Omega \times \Theta}(F_i \times G_j)} |q_{(0,0)}^{(i,j)} \cdots q_{(|\Omega|-1,|\Theta|-1)}^{(i,j)} \rangle |0\rangle_{q_{0_a} \cdots q_{n-1_a}} \\ & + \sum_{q_{(0,0)}^{(i,j)} \cup \dots \cup q_{(0,|\Theta|-1)}^{(i,j)} = 0} \sum_{F_i \times G_j \subseteq \Omega \times \Theta, F_i \subseteq \Omega, G_j \subseteq \Theta} \sqrt{m^{\Omega \times \Theta}(F_i \times G_j)} |q_{(0,0)}^{(i,j)} \cdots q_{(|\Omega|-1,|\Theta|-1)}^{(i,j)} \rangle |1\rangle_{q_{0_a}} |0\rangle_{q_{1_a} \cdots q_{n-1_a}}. \end{aligned}$$

- Perform the X gate on the  $q_{0_a}$ :

$$\begin{aligned} & \sum_{q_{(0,0)}^{(i,j)} \cup \dots \cup q_{(0,|\Theta|-1)}^{(i,j)} = 0} \sum_{F_i \times G_j \subseteq \Omega \times \Theta, F_i \subseteq \Omega, G_j \subseteq \Theta} \sqrt{m^{\Omega \times \Theta}(F_i \times G_j)} |q_{(0,0)}^{(i,j)} \cdots q_{(|\Omega|-1,|\Theta|-1)}^{(i,j)} \rangle |0\rangle_{q_{0_a} \cdots q_{n-1_a}} \\ & + \sum_{q_{(0,0)}^{(i,j)} \cup \dots \cup q_{(0,|\Theta|-1)}^{(i,j)} = 1} \sum_{F_i \times G_j \subseteq \Omega \times \Theta, F_i \subseteq \Omega, G_j \subseteq \Theta} \sqrt{m^{\Omega \times \Theta}(F_i \times G_j)} |q_{(0,0)}^{(i,j)} \cdots q_{(|\Omega|-1,|\Theta|-1)}^{(i,j)} \rangle |1\rangle_{q_{0_a}} |0\rangle_{q_{1_a} \cdots q_{n-1_a}}. \end{aligned}$$

The square of amplitude of  $|1\rangle$  for  $q_{0_a}$  is  $\sum_{\omega_1 \in F_i} m^{\Omega \times \Theta}(F_i \times G_j)$ , which is identical to classical marginalization. The same derivation applies to the other qubits. Hence, the quantum circuits in Definition 11 can implement the marginalization of MFQS without theoretical errors.  $\square$

**Theorem 12.** *The square of amplitude output state  $|m^{\Omega \uparrow \Omega \times \Theta}\rangle$  in Definition 9 equals the outcome of vacuous extension in Eq. (11).*

*Proof.* According to the steps in Definition 9, the specific evolutionary process is:

- The MFQS of  $m^\Omega$  and the ancilla qubits compose the initial state:

$$\sum_{F_i \subseteq \Omega} \sqrt{m^\Omega(F_i)} |\text{bin}(i)\rangle |0\rangle_{q_{(0,0)_a} \cdots q_{(|\Omega|-1,|\Theta|-1)_a}}.$$

- Perform  $|\Theta|$  C-NOT gates on the state, where control bit is  $q_0$ , and target bits are  $q_{(0,0)_a} \cdots q_{(0,|\Theta|-1)_a}$ :

$$\begin{aligned} & \sum_{\omega_1 \in F_i} \sum_{F_i \subseteq \Omega} \sqrt{m^\Omega(F_i)} |\text{bin}(i)\rangle |0\rangle_{q_{(1,0)_a} \cdots q_{(|\Omega|-1,|\Theta|-1)_a}} |1\rangle_{q_{(0,0)_a} \cdots q_{(0,|\Theta|-1)_a}} \\ & + \sum_{\omega_1 \notin F_i} \sum_{F_i \subseteq \Omega} \sqrt{m^\Omega(F_i)} |\text{bin}(i)\rangle |0\rangle_{q_{(0,0)_a} \cdots q_{(|\Omega|-1,|\Theta|-1)_a}}. \end{aligned}$$

- Continue to perform other C-NOT gates:

$$\sum_{F_i \subseteq \Omega} \sqrt{m^\Omega(F_i)} |\text{bin}(i)\rangle \bigotimes_{j=1:|\Omega|} \begin{cases} |1_{|\Theta|}\rangle_{q_{(j-1,0)_a} \cdots q_{(j-1,|\Theta|-1)_a}} & \omega_j \in F_i, \\ |0_{|\Theta|}\rangle_{q_{(j-1,0)_a} \cdots q_{(j-1,|\Theta|-1)_a}} & \omega_j \notin F_i. \end{cases}$$

For a focal set  $F_i$ , the square of amplitude of  $\bigotimes_{j=1:|\Omega|} \begin{cases} |1_{|\Theta|}\rangle_{q_{(j-1,0)_a} \cdots q_{(j-1,|\Theta|-1)_a}} & \omega_j \in F_i, \\ |0_{|\Theta|}\rangle_{q_{(j-1,0)_a} \cdots q_{(j-1,|\Theta|-1)_a}} & \omega_j \notin F_i. \end{cases}$  for  $q_{(0,0)_a} \cdots q_{(|\Omega|-1,|\Theta|-1)_a}$

is  $m^\Omega(F_i)$ , which equals  $m^{\Omega \uparrow \Omega \times \Theta}(F_i \times \Theta)$  in Eq. (11). Hence, the circuit in Definition 9 can implement the vacuous extension without theoretical errors.  $\square$

**Theorem 13.** *The square of amplitude output state  $|m^\Omega[\{\theta_2\}]^{\uparrow\Omega \times \Theta}\rangle$  in Definition 10 equals the outcome of vacuous extension in Eq. (12).*

*Proof.* According to the steps in Definition 10, the specific evolutionary process is:

- The MFQS of  $m^\Omega[F_i]$  and the ancilla qubits compose the initial state:

$$\sum_{G_j \subseteq \Omega} \sqrt{m^\Omega[F_i](G_j)} |\text{bin}(j)\rangle |0\rangle_{q_{(0,0)_a} \cdots q_{(|\Omega|-1, |\Theta|-1)_a}}^{| \Omega \times \Theta |}.$$

- Perform X gates:

$$\sum_{G_j \subseteq \Omega} \sqrt{m^\Omega[F_i](G_j)} |\text{bin}(j)\rangle |\text{bin}(k)\rangle^{| \Omega |},$$

where  $H_k = \Theta \setminus F_i$ .

- Perform C-NOT gates:

$$\sum_{G_j \subseteq \Omega} \sqrt{m^\Omega[F_i](G_j)} |\text{bin}(j)\rangle \bigotimes_{t=1:|\Omega|} \begin{cases} |1_{|\Theta|}\rangle & \omega_t \in G_j, \\ |\text{bin}(k)\rangle & \omega_t \notin G_j. \end{cases}$$

For a focal set  $G_j$ , the square of amplitude of  $\bigotimes_{t=1:|\Omega|} \begin{cases} |1_{|\Theta|}\rangle & \omega_t \in G_j, \\ |\text{bin}(k)\rangle & \omega_t \notin G_j. \end{cases}$  for  $q_{(0,0)_a} \cdots q_{(|\Omega|-1, |\Theta|-1)_a}$  is  $m^\Omega[F_i](G_j)$ ,

which equals  $m^\Omega[F_i]^{\uparrow\Omega \times \Theta}(F_i \times G_j \cup \Omega \times \overline{F_i})$  in Eq. (12). Hence, the circuit in Definition 12 can implement the ballooning extension without theoretical errors.

□
